# Supplementary material for: Application of NotebookLM, a Large Language Model with Retrieval-Augmented Generation, for Lung Cancer Staging
Source: arXiv:2410.10869 ancillary file (2024-10-08)
Supplement: Supplementary file 2 [file OnlineResource2.pdf]

[TNM classification of lung cancer in Japan, 8th edition]

T—Primary Tumor

TX: Presence of the primary tumor cannot be assessed, or positive cytology is observed only in sputum or bronchial lavage, and the tumor cannot be observed by imaging or bronchoscopy.

T0: No evidence of primary tumor.

Tis: (This classification is referred to as carcinoma in situ.) The diameter of the solid component is 0 cm and the overall lesion (ground-glass nodule) diameter is less than or equal to 3 cm.

T1: The diameter of the solid component is less than or equal to 3 cm, covered by lung or visceral pleura, with no invasion proximal to the lobar bronchus observed by bronchoscopy (i.e., not involving the main bronchus).

T1 includes the subclasses T1mi, T1a, T1b, and T1c, which must meet the following criteria in addition to the T1 criteria.

T1mi: The solid component diameter is greater than 0 cm and less than or equal to 0.5 cm and the overall lesion (ground-glass nodule) diameter is less than or equal to 3 cm.

T1a: The solid component diameter is less than or equal to 1 cm and does not meet the criteria for Tis or T1mi.

T1b: Solid component diameter greater than 1 cm and less than or equal to 2 cm.

T1c: Solid component diameter greater than 2 cm and less than or equal to 3 cm.

T2: Solid component diameter greater than 3 cm and less than or equal to 5 cm, or a solid component diameter less than or equal to 3 cm with any of the following: 1. Involvement of the main bronchus without involvement of the carina. 2. Invasion of the visceral pleura. 3. Partial or complete atelectasis or obstructive pneumonitis extending to the pulmonary hilum.

T2 includes the subclasses T2a and T2b, which must meet the following criteria in addition to the T2 criteria.

T2a: Solid component diameter greater than 3 cm and less than or equal to 4 cm.

T2b: Solid component diameter greater than 4 cm and less than or equal to 5 cm.

T3: Solid component diameter greater than 5 cm and less than or equal to 7 cm, or a solid component diameter less than or equal to 5 cm with any of the following: 1. Direct invasion of the parietal pleura, chest wall (including superior sulcus tumor), phrenic nerve, or pericardium. 2. Separate tumor nodule(s) in the same lung lobe as the primary tumor.

T4: Meets one of the following conditions. 1. Solid component diameter greater than 7 cm. 2. Tumor invasion of the diaphragm, mediastinum, heart, great vessels, trachea, recurrent laryngeal nerve, esophagus, vertebral body, or carina. 3. Separate tumor nodule(s) in a different ipsilateral lobe from the primary tumor.

#### N—Regional Lymph Nodes

NX: Regional lymph nodes cannot be assessed.

N0: No regional lymph node metastasis.

N1: Metastasis in ipsilateral peribronchial and/or ipsilateral hilar lymph nodes from the primary tumor, including direct extension of the primary tumor.

N2: Metastasis in ipsilateral mediastinal lymph nodes from the primary tumor and/or in subcarinal lymph nodes.

N3: Metastasis in contralateral mediastinal, contralateral hilar, ipsilateral or contralateral scalene, or supraclavicular lymph nodes from the primary tumor.

#### M—Distant Metastasis

M0: No distant metastasis.

M1a: Separate tumor nodule(s) in the contralateral lung from the primary tumor, pleural or pericardial nodules, malignant pleural effusion (ipsilateral or contralateral), or malignant pericardial effusion.

M1b: Single metastasis outside the lungs.

M1c: Multiple metastases outside the lungs.

[Additional Information]

A pure ground-glass nodule exceeding 3 cm is classified as T1a.

Tumor invasion confined to the bronchial wall is classified as T1a.

Tumors that meet the criteria for T2 but are 3 cm or less in size are classified as T2a.

In the T4 classification, major vessels refer to the aorta, superior vena cava, inferior vena cava, main pulmonary artery (pulmonary trunk), pulmonary veins and arteries within the pericardium, brachiocephalic veins and artery, subclavian veins and arteries, and the left common carotid artery.

Invasion of the pericardium is classified as T3, but invasion of the epicardium, like invasion of the heart, is classified as T4.

Brachial plexus invasion above the C8 level is classified as T4.

In the presence of carcinomatous lymphangitis, if it is confined to the same lung lobe but not contiguous with the primary lung cancer, it is classified as T3; if found in a different lobe of the ipsilateral lung, it is classified as T4; if found in the contralateral lung, it is classified as M1a.

If there are non-contiguous metastases on the chest wall or diaphragm outside the parietal pleura, they are classified as M1b if single, and M1c if multiple.

Distant lymph node metastasis outside of the regional lymph nodes (i.e., not classified as N1, N2, or N3) is classified as M1b if single, and M1c if multiple.

Note that, when the primary lung tumor is located in the left lung, ipsilateral refers to the left side and contralateral refers to the right side. Conversely, when the primary lung tumor is in the right lung, ipsilateral refers to the right side and contralateral refers to the left side.
